# Supplementary material for: Tuning Mixed Input Hyperparameters on the Fly for Efficient Population Based AutoRL
Source: arXiv:2106.15883 source file (2021-06-30)
Supplement: Supplementary file 1 [file appendix_rlbackground.tex]

\section{Reinforcement Learning Algorithm Detail}
